# Supplementary material for: Combining micro- and macroscopic probes to untangle single-ion and spatial exchange anisotropies in a $S = 1$ quantum antiferromagnet
Source: arXiv:1611.06971 source file (2016-11-21)
Supplement: Supplementary file 1 [file NiSbF6Supplementary.pdf]

# Supplementary Information

## Combining Micro- and Macroscopic Probes to Untangle Single-Ion and Spatial Exchange Anisotropies in a $S = 1$ Quantum Antiferromagnet

*Jamie Brambleby,[1] Jamie L. Manson,[2,3*] Paul A. Goddard,[1] Matthew B. Stone,[4] Roger D. Johnson,[5,6] Pascal Manuel,[6] Jacqueline A. Villa,[2] Craig M. Brown,[3] John Singleton,[7] Shalinee Chikara,[7] Vivien Zapf,[7] Helen Lu, [7] Saul H. Lapidus,[8] Rebecca Scatena,[9] Piero Macchi,[9] Yu-sheng Chen[10] and Lai-Chin Wu[10]*

[1]*Department of Physics, University of Warwick, Coventry CV4 7AL, UK*

[2]*Department of Chemistry and Biochemistry, Eastern Washington University, Cheney, WA 99004, USA*

[3]*NIST Center for Neutron Research, National Institute of Standards and Technology, Gaithersburg, MD 20899, USA*

[4]*Quantum Condensed Matter Division, Oak Ridge National Laboratory, Oak Ridge, TN 37831, USA*

[5]*Clarendon Laboratory, Department of Physics, University of Oxford, Oxford OX1 3PU, UK*

[6]*ISIS Pulsed Neutron Source, STFC Rutherford Appleton Laboratory, Didcot, Oxfordshire OX11 0QX, UK*

[7]*National High Magnetic Field Laboratory, Los Alamos National Laboratory, Los Alamos, NM 8754, USA*

[8]*X-ray Sciences Division, Advanced Photon Source, Argonne National Laboratory, Argonne, IL 60439, USA*

[9]*Department of Chemistry and Biochemistry, University of Bern, 3012 Bern, Switzerland*

[10]*ChemMatCARS, Advanced Photon Source, Argonne National Laboratory, Argonne, IL 60439, USA*

*Phone: (509) 359-2878; fax: (509) 359-6973; e-mail: jmanson@ewu.edu

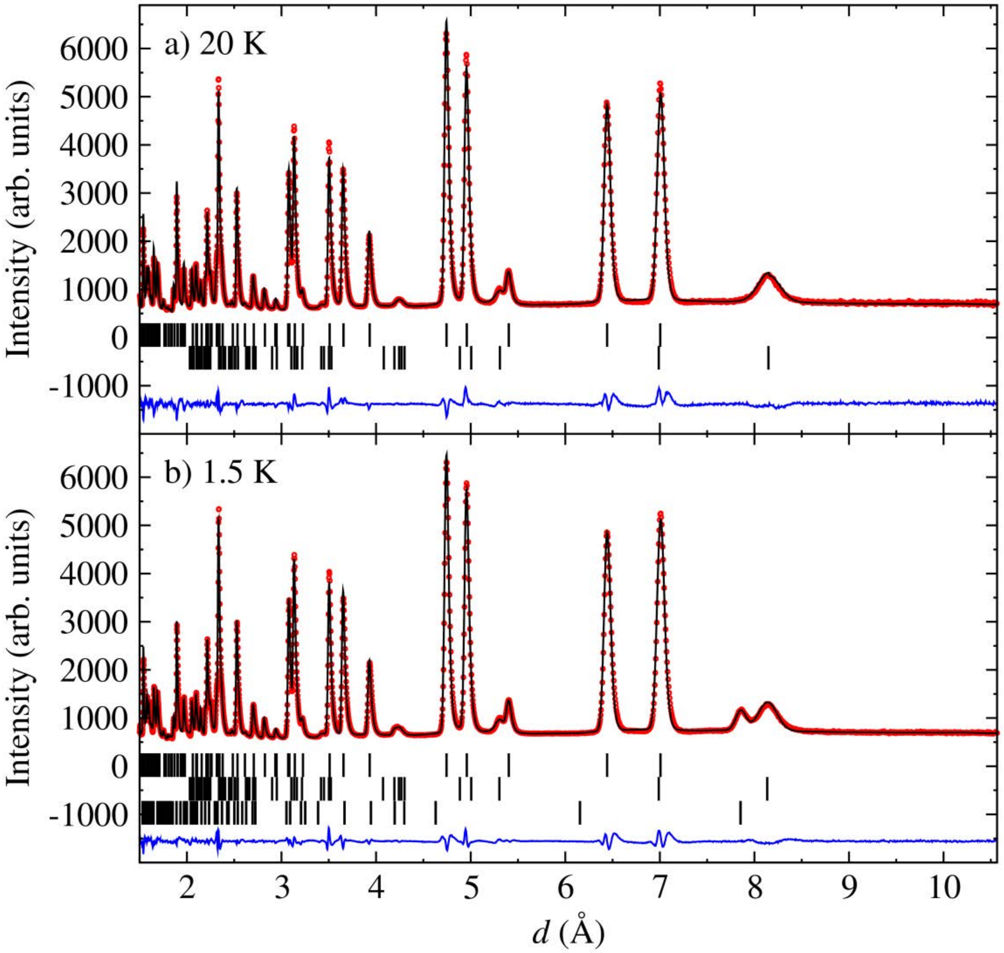


**Fig. S1**. Refinement of neutron powder diffraction data for $[Ni(HF_2)(pyz\text{-}d_4)_2]SbF_6$ at (a) 20 K and (b) 1.5 K. WISH Bank 2 data (red points), Rietveld fitted model (black line), reflections of the *P*4/*nmm* lattice (black ticks, top line), reflections of the magnetic moments with propagation vector $k$ = (0,0,1/2) (black ticks, bottom line) and $I_{obs}$ - $I_{calc}$ (blue line). The bottom row (20 K) and middle row (1.5 K) of ticks in each plot indicate structural peaks due to a 1.6% co-crystallized impurity of $[Ni(pyz)_2(H_2O)_2]F{\cdot}SbF_6$ (orthorhombic; *Ibam*) as determined by LeBail profile matching.

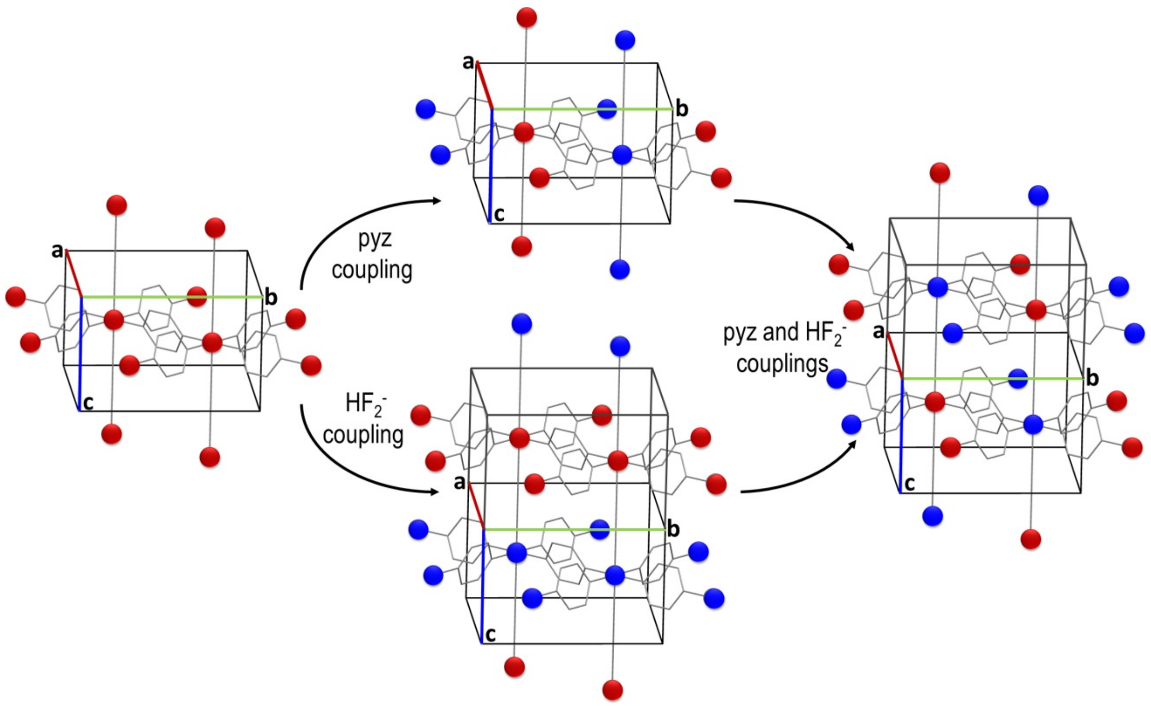


**Fig. S2**. Models used in the DFT calculation of the *J* and *J*' exchange interactions. We consider an FM state and two different AFM states, with spin pairing along the *c*-axis ($AFM_{FHF}$) or in the *ab*-plane ($AFM_{pyz}$), as well as the fully AFM state featuring both kinds of pairing.
